# Supplementary material for: Human Parity on CommonsenseQA: Augmenting Self-Attention with External Attention
Source: arXiv:2112.03254 source file (2022-05-04)
Supplement: Supplementary file 1 [file appendix.tex]

\newpage
\appendix

\section{Datasets}
We use a combination of 17 datasets for our largest-scale training data retrieval. 

% The datasets include 
\noindent$\alpha$NLI \citep{bhagavatula2019abductive} is a natural language inference dataset testing a model's ability on abductive reasoning and common sense, and is formulated as a binary classification task.\\ 
SWAG \citep{zellers2018swagaf} is a dataset for studying grounded commonsense inference and the model needs to predict what will happen next after a given situation. \\
RACE \citep{lai2017large} is a reading comprehension dataset with questions from English language exams in China. We only use the middle school subset in RACE. \\
CODAH \citep{chen2019codah} is of a similar format as SWAG, but is adversarially constructed by human to make it challenging.\\
RiddleSense \citep{lin2021riddlesense} consists of riddle questions to test a model's commonsense reasoning capability. \\
SciTail \citep{scitail} is an entailment dataset focusing on science question answering. \\
Com2Sense \citep{singh2021com2sense} is a adversarially designed dataset comprising true/false statements about common sense. \\
AI2 Science Questions \citep{clark2019f} consists of questions from student assessments in elementary and middle schools in the US.\\
WinoGrade \citep{sakaguchi2019winogrande} is an adversarial winograd schema challenge on coreference resolution in slot filling style. \\
CommonsenseQA2.0 \citep{talmor2021commonsenseqa} is the new version of CommonsenseQA with yes/no questions on everyday commonsense knowledge. \\
ASQ \citep{fu2019asking} focuses on advise-seeking conversations; the model needs to pick the correct question by reading the answer to it.\\
OBQA \citep{OpenBookQA2018} has questions from open-book exams on elementary-level science questions. \\
PhysicalIQA \citep{Bisk2020} is a QA benchmark for naive physics reasoning on how people interact with everyday objects in everyday situations. \\
SocialIQA\citep{Sap2019SocialIC} is a QA benchmark on social commonsense intelligence, focusing on people's actions and their social implications.\\
CosmosQA \citep{huang2019cosmos} is a reading comprehension dataset that requires commonsense to reason about likely causes/effects.\\ 
HellaSWAG \citep{zellers2019hellaswag} is a dataset for studying grounded commonsense inference similar to SWAG, but with adversarially filtering to make it more difficult.

% (we only use the middle-school subset), CODAH , RiddleSense \citep{lin2021riddlesense}, SciTail \citep{scitail}, Com2Sense \citep{singh2021com2sense}, AI2 Science Questions \citep{clark2019f}, WinoGrade \citep{sakaguchi2019winogrande}, CommonsenseQA \citep{talmor2018commonsenseqa}, CommonsenseQA2.0 \citep{talmor2021commonsenseqa}, ASQ \citep{fu2019asking}, OBQA \citep{OpenBookQA2018}, PhysicalIQA \citep{Bisk2020}, SocialIQA\citep{Sap2019SocialIC}, CosmosQA \citep{huang2019cosmos} and HellaSWAG \citep{zellers2019hellaswag}.
% We present details of the datasets that we use for training data retrieval in Table \ref{tab:datasets}.
% \begin{table}[th]
% 	\centering
% 	\begin{tabular}{lccc}
% 		\thickhline
% 		\textbf{Dataset}& \textbf{Task} & \textbf{\#Train} & \textbf{\#Label} \\
% 		\hline
% 		$\alpha$NLI & NLI & 170k & 2\\
% 		SWAG & MC & 73.5k & 4\\
% 		RACE-Middle & MRC & 87.9k & 4\\
% 		CODAH & MC & 1672 & 4\\
% 		RiddleSense & MC & 3512 & 5\\
% 		SciTail & NLI & 23.6k & 2\\
% 		Com2Sense & MC & 808& 2\\
% 		AI2Science & MC & 1232 & 4\\
% 		WinoGrade & CoRef & 40.4k & 2\\
% 		CSQA & MC & 9741 & 5\\
% 		CSQA2.0 & CLF & 9264 & 2\\
% 		ASQ & MC & 8872 & 2\\
% 		OBQA & MC & 4960 & 4\\
% 		PhysicalIQA & MC & 16.1k & 2\\
% 		SocialIQA & MC & 33.4k & 3\\
% 		CosmosQA & MRC & 25.3k & 4\\
% 		HellaSWAG & NSP & 39.9k & 4\\
% 		\thickhline
% 	\end{tabular}
% 	\caption{\label{tab:datasets} The datasets used for training data retrieval. NLI stands for natural language inference, MC is multiple choice, MRC is machine reading comprehension, CLF is classification, NSP is next sentence prediction.}
% \end{table}
